# Supplementary material for: ViLMA: A Zero-Shot Benchmark for Linguistic and Temporal Grounding in Video-Language Models
Source: arXiv:2311.07022 source file (2023-11-13)
Supplement: Supplementary file 1 [file appendix_evaluation.tex]

\section{Evaluation Metrics}
\label{sec:appendix:eval_metrics}
Following \citet{parcalabescu-etal-2022-valse}, we use 5 
metrics: (i) overall \textbf{accuracy} ($acc$) using both captions and foils as  classes; (ii) caption \textbf{precision} ($p_c$) 
and (iii) \textbf{foil precision} ($p_f$);
(iv) \textbf{area under the receiver operating characteristic curve} (AUROC);
and (v) \textbf{pairwise ranking accuracy} ($acc_r$).
Pairwise accuracy is utilised to measure the model's proficiency in discerning between different visual scenarios, capturing its ability to make accurate pairwise distinctions. The area under the receiver operating characteristic curve (AUROC) provides insights into the model's discriminative capabilities across a range of operating points. Overall accuracy offers a holistic view of the model's correctness in predicting both caption and foil instances. Caption precision delves into the model's accuracy specifically in generating relevant captions, while foil precision scrutinises the model's ability to avoid generating misleading captions. This multifaceted approach to evaluation ensures a better understanding of the model's strengths and weaknesses, contributing to a more thorough and insightful assessment of its performance on \dataset{}.
